# Supplementary material for: ClinicalGPT: Large Language Models Finetuned with Diverse Medical Data and Comprehensive Evaluation
Source: arXiv:2306.09968 source file (2023-06-16)
Supplement: Supplementary file 1 [file supplementary.tex]

% % \documentclass{article}
% \documentclass[UTF8]{article}
  
% %% Title
% \title{Supplementary
% %%%% Cite as
% %%%% Update your official citation here when published 
% % \thanks{\textit{\underline{Citation}}: 
% % \textbf{Authors. Title. Pages.... DOI:000000/11111.}} 
% }

% \begin{document}
% \maketitle
% \subsection{}

% \end{document}
